# Supplementary material for: Turbulence statistics in a 2D vortex condensate
Source: arXiv:1711.05536 source file (2017-11-15)
Supplement: Supplementary file 1 [file vortexfluc-sm.pdf]

# Turbulence statistics in a 2D vortex condensate — Supplementary Material

Anna Frishman[1,2,*] and Corentin Herbert[3,2,†]

[1] *Princeton Center for Theoretical Science, Princeton University, Princeton, New Jersey 08544, USA*
[2] *Department of Physics of Complex Systems, Weizmann Institute of Science, P.O. Box 26, 76100 Rehovot, Israel*
[3] *Univ Lyon, ENS de Lyon, Univ Claude Bernard, CNRS, Laboratoire de Physique, F-69342 Lyon, France*

* frishman@princeton.edu
† corentin.herbert@ens-lyon.fr

| Run | $K_f \equiv L/\ell_f$ | $\delta \equiv \alpha L^{2/3} \varepsilon^{-1/3}$ | $R_u/L \equiv \delta^{-1/2} K_f^{-2/3}$ | $\Gamma \equiv \nu K_f^p/\alpha$ |
|---|---|---|---|---|
| Z | 100 | $1.23 \cdot 10^{-2}$ | 0.12 | 25 |
| A | 100 | $8.14 \cdot 10^{-3}$ | 0.15 | 45.5 |
| B | 100 | $4.58 \cdot 10^{-3}$ | 0.2 | 90.9 |
| C | 100 | $2.4 \cdot 10^{-3}$ | 0.28 | 200 |
| D | 100 | $1.45 \cdot 10^{-3}$ | 0.36 | 400 |
| E | 100 | $1.09 \cdot 10^{-3}$ | 0.41 | 800 |

TABLE SI. Non-dimensional parameters for the runs discussed in the main text.

## SI. ADDITIONAL DETAILS ABOUT THE NUMERICAL SIMULATIONS

Here, we provide additional information about the numerical simulations discussed in the main text.

First, non-dimensional parameters characterizing the runs are summarized in Table SI. This includes in particular the small parameter $\delta \ll 1$ measuring the timescale separation between the mean-flow (the pair of vortices forming the condensate, see Fig. 1 in the main text) and turbulent fluctuations, the forcing scale $K_f \gg 1$ and the estimated size of the universal region $R_u$. When the latter reaches a sizeable fraction of the box size $L$, we expect boundaries (or here, the presence of the other vortex) to become important. In the case under study, the domain has a finite diameter (the largest distance between any two points) $L/\sqrt{2} \approx 0.7L$. Hence, already for $R_u > 0.35L$, which is the case for runs D and E, the regions for the two vortices of opposite sign necessarily collide. For this reason, we take a conservative approach and define the region where we expect the quasi-linear theory to hold *a priori* as $K_f \leq r/L \leq R_u^{(A)} \approx 0.15$. This is the shaded region in the figures. Fig. S1 shows the vorticity and velocity profile for the mean-flow, rescaled

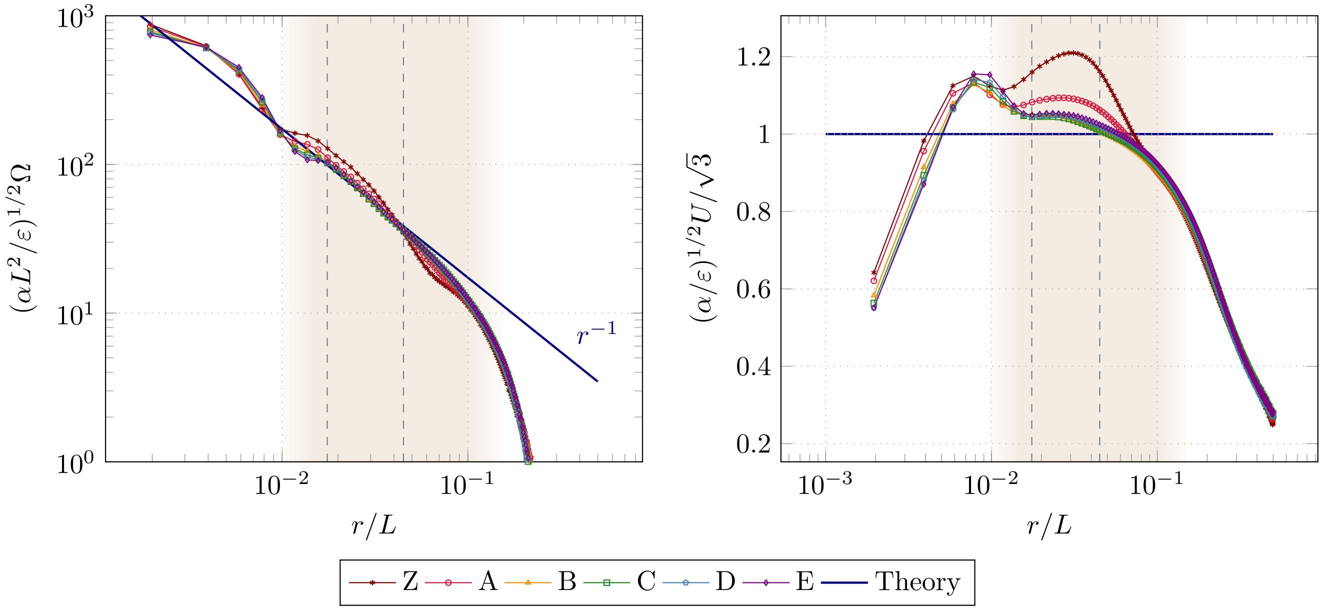


FIG. S1. (color online) Vorticity (left) and velocity (right) profiles for the mean-flow, rescaled by the theoretical predictions [1].

according to the theoretical prediction [1]: $U = \sqrt{3\varepsilon/\alpha}, \Omega = U/r$ (see main text). As discussed in the main text, the region where the theoretical predictions hold in practice is narrower than the shaded region, and we indicate it approximately with dashed vertical lines.

In Fig. S2, we plot the decomposition of the azimuthal and radial components of turbulent energy into angular harmonics (see main text and section SII A) $m = 0, \dots, 5$ for run E. This makes it clear that both $u$ and $v$ are overwhelmingly dominated by the $m = 1$ mode in the region of interest, and even in the vortex core. The $m = 3$ harmonics prevails outside that region, in the region where the mean-flow is weak. We also check that the $m = 0$ mode is very small for $v$, as it should from incompressibility. Similar results hold for the other runs. Fig. S3 shows the raw data for the angular harmonics profiles, rescaled only by the Kolmogorov estimate for turbulent energy level. As explained in the main text, this rescaling does not suffice to explain the behavior of turbulent fluctuations in

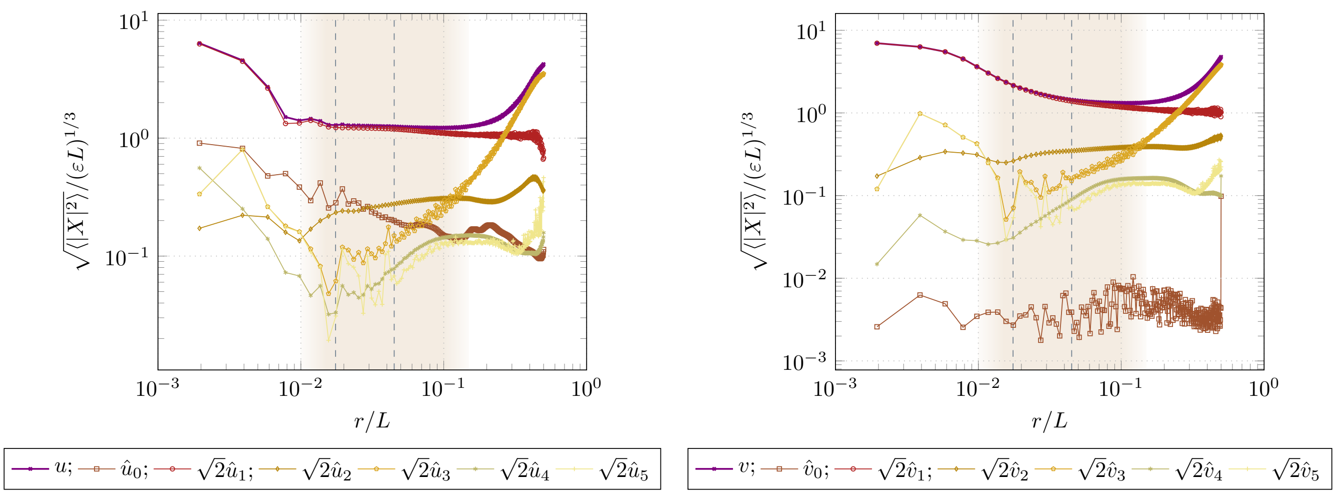


FIG. S2. (color online) Breakup of the turbulent energy profiles $\langle u^2\rangle$ and $\langle v^2\rangle$ into contributions by the angular harmonics $0 \le m \le 5$.

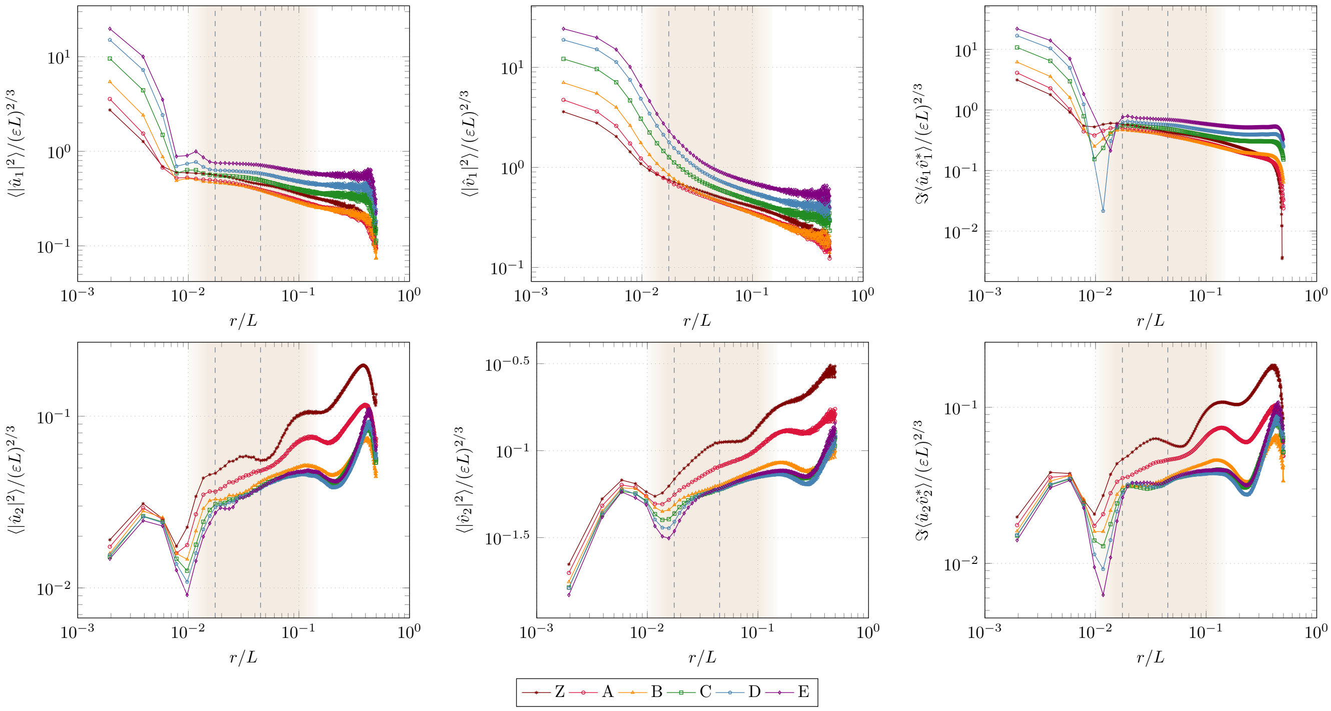


FIG. S3. (color online) The profile of the first two angular harmonics $m = 1$ (top row) and $m = 2$ (bottom row) of turbulent energy, for all the runs.

the presence of the mean-flow. Note, however, that it performs much better for the higher-order harmonics (only $m = 2$ is shown here but our data indicate that it remains true for higher orders) than for $m = 1$ (which dominates the turbulent energy profile). We reconstruct these profiles based on zero modes of the advection equation for the two-point correlation functions in sections SII E and SII F.

## SII. THEORETICAL RESULTS FOR THE VELOCITY COVARIANCE ANGULAR HARMONICS

### A. Derivation of the Lyapunov equation

Our aim is to derive the advection equation for the velocity two-point correlation function. This can be done by deriving an equation for the vorticity covariance, and then using that $\omega = \nabla \times \mathbf{v}$ to express it in terms of the velocity, as explained in the main text. In this way one does not need to deal with the pressure explicitly. The other option, which we present here, is to derive directly an equation for the velocity covariance, and then act on it with a differential operator to express the pressure in terms of the velocity.

We begin with the expression for $\partial_t \langle v^i(\mathbf{r_1}) v^j(\mathbf{r_2})\rangle$, with the notations of the main text $\mathbf{v} = \langle \mathbf{v}\rangle + \tilde{\mathbf{v}}$. We will use the same notation for the pressure field. We have

$$\langle v_1^l \nabla_1^l v_1^i v_2^j\rangle + \langle v_2^l \nabla_2^l v_2^j v_1^i\rangle + \langle \nabla_1^i p_1 v_2^j\rangle + \langle \nabla_2^j p_2 v_1^i\rangle = \langle f_1^i v_2^j\rangle + \langle f_2^j v_1^i\rangle - 2\alpha \langle v^i(\mathbf{r_1}) v^j(\mathbf{r_2})\rangle, \tag{S1}$$

in the steady state — ignoring the (hyper)viscosity for the moment.

Next, the average of the momentum balance equation multiplied by the mean velocity gives the equation for the energy balance in the mean flow

$$\langle v_1^l \nabla_1^l v_1^i\rangle \langle v_2^j\rangle + \langle v_2^l \nabla_2^l v_2^j\rangle\langle v_1^i\rangle + \langle \nabla_1^i p_1\rangle\langle v_2^j\rangle + \langle \nabla_2^j p_2\rangle\langle v_1^i\rangle = -2\alpha \langle v^i(\mathbf{r_1})\rangle\langle v^j(\mathbf{r_2})\rangle, \tag{S2}$$

where we assumed that $\langle \mathbf{f}\rangle = 0$. Then, subtracting (S2) from (S1), one gets

$$\begin{aligned}&\langle \tilde{v}_2^j \tilde{v}_1^l\rangle \nabla_1^l \langle v_1^i\rangle + \langle \tilde{v}_1^i \tilde{v}_2^l\rangle \nabla_2^l \langle v_2^j\rangle + \left(\langle v_1^l\rangle \nabla_1^l + \langle v_2^l\rangle \nabla_2^l\right)\langle \tilde{v}_1^i \tilde{v}_2^j\rangle + \langle \tilde{v}_2^j \tilde{v}_1^l \nabla_1^l \tilde{v}_1^i\rangle + \langle \tilde{v}_1^i \tilde{v}_2^l \nabla_2^l \tilde{v}_2^j\rangle + \langle \nabla_1^i \tilde{p}_1 \tilde{v}_2^j\rangle + \langle \nabla_2^j \tilde{p}_2 \tilde{v}_1^i\rangle \\ &= \langle f_1^i \tilde{v}_2^j\rangle + \langle f_2^j \tilde{v}_1^i\rangle - 2\alpha\langle \tilde{v}_1^i \tilde{v}_2^j\rangle.\end{aligned} \tag{S3}$$

In cylindrical coordinates, in the radial direction, direction $i = j = \hat{r}$ we get

$$\begin{aligned}\left(\frac{U}{r_1} - \frac{U}{r_2}\right)\partial_{\phi_1}\langle v_1 v_2\rangle + \partial_{r_1}\langle v_2 p_1\rangle + \partial_{r_2}\langle v_1 p_2\rangle = &- \langle (\tilde{\mathbf{v}}_\mathbf{1}^l \nabla_1^l \tilde{\mathbf{v}}_\mathbf{1})_r v_2\rangle - \langle (\tilde{\mathbf{v}}_\mathbf{2}^l \nabla_2^l \tilde{\mathbf{v}}_\mathbf{2})_r v_1\rangle + \frac{2U}{r_1}\langle u_1 v_2\rangle + \frac{2U}{r_2}\langle u_2 v_1\rangle \\ &+ 2\chi_{12}^{rr} - 2\alpha\langle v_1 v_2\rangle,\end{aligned} \tag{S4}$$

where we assumed that the mean flow, $U(r)$, is purely in the azimuthal direction. Note that the terms $\langle \tilde{v}_2^j \tilde{v}_1^l\rangle \nabla_1^l \langle v_1^i\rangle + \langle \tilde{v}_1^i \tilde{v}_2^l\rangle \nabla_2^l \langle v_2^j\rangle$ are non-zero for $i = j = \hat{r}$ due to the metric terms in the convective derivative, they contribute $-\frac{U}{r_1}\langle u_1 v_2\rangle - \frac{U}{r_2}\langle u_2 v_1\rangle$. We have used the definition $\langle f_1^i(t) f_2^j(t')\rangle = 2\delta(t-t')\chi_{12}^{ij}$.

The pressure can be expressed in the form

$$-\nabla^2 p = -\frac{1}{r}\partial_r U^2 + \frac{1}{r}\partial_r U(2\partial_\phi v - 2u) - \frac{2U}{r}\partial_r u + \frac{1}{r}\partial_r(r\partial_r v^2) + \frac{2}{r^2}\partial_r\partial_\phi(ruv) + \frac{1}{r}\partial_r(v^2 - u^2) + \frac{1}{r^2}\partial_\phi^2 u^2. \tag{S5}$$

The profile, $U$, that was found in [1] is independent of the radius so that one has

$$-\nabla^2 p = -\frac{2U}{r}\partial_r u + \frac{1}{r}\partial_r(r\partial_r v^2) + \frac{2}{r^2}\partial_r\partial_\phi(ruv) + \frac{1}{r}\partial_r(v^2 - u^2) + \frac{1}{r^2}\partial_\phi^2 u^2. \tag{S6}$$

We will use this formula to express the pressure in equation (S4) in terms of the velocity correlation functions. For this purpose, we multiply equation (S4) by $r_1 r_2$ and then act on it with $r_1^2\Delta_1 r_2^2\Delta_2$ (since $r^2\nabla^2 = (r\partial_r)^2 + \partial_\phi^2$ commutes with $r\partial r$ and $\partial_\phi$ we can then use the identity for the pressure, (S6)). As the three types of velocity two point, second order, correlation functions are related via incompressibility: $\partial_{\phi_1}\partial_{\phi_2}\langle u_1 u_2\rangle = \partial_{r_1} r_1 \partial_{r_2} r_2 \langle v_1 v_2\rangle$, $\partial_{\phi_1}\langle v_2 u_1\rangle = -\partial_{r_1} r_1 \langle v_2 v_1\rangle$, we do not need to solve them simultaneously, but rather can express the two other correlation functions in terms of $\langle v_1 v_2\rangle$. Denote $\mathcal{L}_{12} = r_1^2\nabla_1^2 r_2^2 \nabla_2^2$, $\mathcal{L}_i = r_i^2\nabla_i^2$. We use $(\tilde{\mathbf{v}}^l\nabla^l\tilde{\mathbf{v}})_r = \frac{1}{r}\partial_r(rv^2) + \frac{1}{r}\partial_\phi uv - \frac{uv}{r}$ and the identity (S6) for pressure, to obtain

$$\begin{aligned}&\mathcal{L}_{12} U (r_2 - r_1)\partial_{\phi_1}\langle v_1 v_2\rangle + 2U\mathcal{L}_2 r_2 (r_1\partial_{r_1})^2\langle v_2 u_1\rangle - \mathcal{L}_2 r_2 (r_1\partial_{r_1})^3\langle v_2 v_1^2\rangle - 2\mathcal{L}_2 r_2 r_1 \partial_{r_1} r_1 \partial_{\phi_1}\langle v_2 v_1 u_1\rangle \\ &- \mathcal{L}_2 r_2 (r_1\partial_{r_1})^2\partial_{\phi_1}\langle v_2(v_1^2 - u_1^2)\rangle - \mathcal{L}_2 r_2 r_1 \partial_{r_1}\partial_{\phi_1}^2\langle v_2 u_1^2\rangle\rangle + (1 \leftrightarrow 2) = -\mathcal{L}_{12} r_2 \partial_{r_1} r_1 \langle v_1^2 v_2\rangle - \mathcal{L}_{12} r_1 \partial_{r_2} r_2 \langle v_2^2 v_1\rangle \\ &- \mathcal{L}_{12} r_2 \partial_{\phi_1}\langle u_1 v_2 v_1\rangle - \mathcal{L}_{12} r_1 \partial_{\phi_2}\langle u_2 v_2 v_1\rangle - \mathcal{L}_{12} r_2 \langle u_1 v_1 v_2\rangle - \mathcal{L}_{12} r_1 \langle u_2 v_1 v_2\rangle + 2U\mathcal{L}_{12} r_2\langle u_1 v_2\rangle + 2U\mathcal{L}_{12} r_1 \langle u_2 v_1\rangle + \\ &+ 2\mathcal{L}_{12} r_2 r_1 \chi_{12}^{rr} - 2\mathcal{L}_{12} r_2 r_1 \alpha\langle v_1 v_2\rangle.\end{aligned} \tag{S7}$$

Now we make the quasi-linear approximation, assuming that cubic terms in the velocity are negligible, resulting in

$$\mathcal{L}_{12}U\left(r_2-r_1\right)\partial_{\phi_1}\langle v_1v_2\rangle-2U\mathcal{L}_2r_2\partial^2_{\phi_1}\langle v_2u_1\rangle+-2U\mathcal{L}_1r_1\partial^2_{\phi_2}\langle v_1u_2\rangle=2\mathcal{L}_{12}r_2r_1\chi^{rr}_{12}-2\mathcal{L}_{12}r_2r_1\alpha\langle v_1v_2\rangle. \tag{S8}$$

Finally, we use incompressibility $\partial_{\phi_1}\langle v_2u_1\rangle=-\partial_{r_1}r_1\langle v_2v_1\rangle$, to obtain :

$$U\left[-\mathcal{L}_1r_1\left(2\partial_{r_2}r_2+\mathcal{L}_2\right)\partial_{\phi_1}+\mathcal{L}_2r_2\left(2\partial_{r_1}r_1+\mathcal{L}_1\right)\partial_{\phi_1}+2\frac{\alpha}{U}\mathcal{L}_{12}r_2r_1\right]\langle v_1v_2\rangle=2\mathcal{L}_{12}r_1r_2\chi^{rr}_{12}. \tag{S9}$$

Neglecting the effects of friction and forcing, we arrive at equation (3) in the main text.

In the main text we focus on the (angular) Fourier modes of the two point correlation function, by isotropy,

$$\langle v_1v_2\rangle=\sum_{m=-\infty}^{\infty}\langle\hat{v}_m(r_1)\hat{v}^*_m(r_2)\rangle e^{im\Delta\phi},\qquad\text{where }\hat{v}_m(r)=\frac{1}{2\pi}\int_{-\pi}^{\pi}v(r,\phi)e^{-im\phi}d\phi. \tag{S10}$$

We note that, if we keep the forcing term, the Fourier modes of the forcing two point correlation function would be suppressed by a factor of at least $\min(l_f/r_1,l_f/r_2)$, the maximal range of angles that has a non-vanishing contribution to the integral. However, for $r_1\to r_2$ the leading order of the convective operator also turns to zero and the forcing term becomes important for small enough radial separations. In any case, we will assume that (the harmonics of) velocity correlation functions are continuous in the limit of $l_f/L\to 0$ and then $r_1\to r_2$, and will neglect the contribution from the forcing.

## B. Scale-invariant solutions of the homogeneous Lyapunov equation

### 1. The general case

Let us analyze the solutions of the Hypergeometric equation, equation (4) in the main text:

$$\prod_{i=1}^{4}\left(R\frac{d}{dR}-\gamma_i\right)f_m(R)=R\prod_{i=1}^{4}\left(R\frac{d}{dR}+\alpha_i\right)f_m(R), \tag{S11}$$

where $(\gamma_1,\gamma_2,\gamma_3,\gamma_4)=(-1-\sqrt{m^2-1},-1+\sqrt{m^2-1},\bar{\lambda}-m,\bar{\lambda}+m)$, $(\alpha_1,\alpha_2,\alpha_3,\alpha_4)=(1-m,1+m,-\bar{\lambda}+\sqrt{m^2-1},-\bar{\lambda}-\sqrt{m^2-1})$. This is a fourth order ODE with three regular singular points at $R=0,\infty,1$

The solutions of (S11) can be expressed as a Frobenius series around $R=0$ (or $1/R=0$), resulting in the generalized Hypergeometric functions as solutions: $f^s_m(R)=R^{\gamma_s}{}_4F_3(a^s_1,a^s_2,a^s_3,a^s_4;b^s_1,b^s_2,b^s_3;R)$, where

$${}_4F_3\left(a_1,a_2,a_3,a_4;b_1,b_2,b_3;R\right)=\sum_{k=0}^{\infty}\frac{R^k\left(a_1\right)_k\left(a_2\right)_k\left(a_3\right)_k\left(a_4\right)_k}{k!\left(b_1\right)_k\left(b_2\right)_k\left(b_3\right)_k},\qquad\text{with }\left(a\right)_k=a(a+1)\cdots(a+k-1). \tag{S12}$$

The above expression for ${}_4F_3$ is invariant under permutation of the $a_i$ (resp. $b_i$), hence the order does not matter. The parameters are given by $\{a^s_i\}_{1\le i\le 4}=\{\gamma_s+\alpha_i\}_{1\le i\le 4}$ and $\{b^s_i\}_{1\le i\le 3}=\{\gamma_s-\gamma_i+1\}_{i\neq s}$. The representation around $1/R=0$, is obtained by interchanging $\alpha$ and $\gamma$ and $R\to 1/R$: $f^s_m(R)=R^{\alpha_s}{}_4F_3(a^s_1,a^s_2,a^s_3,a^s_4;b^s_1,b^s_2,b^s_3;1/R)$ where $\{a^s_i\}_{1\le i\le 4}=\{\gamma_s+\alpha_i\}_{1\le i\le 4}$ and $\{b^s_i\}_{1\le i\le 3}=\{\alpha_s-\alpha_i+1\}_{i\neq s}$ [2].

The resulting parameters for the four solutions around $R=0$ ($R<1$) are the following, denoting $S\equiv\sqrt{m^2-1}$,

| $s$ | $\gamma_s$ | $a^s_1$ | $a^s_2$ | $a^s_3$ | $a^s_4$ | $b^s_1$ | $b^s_2$ | $b^s_3$ |
|---|---|---|---|---|---|---|---|---|
| 1 | $-1-S$ | $-S-m$ | $m-S$ | $-\bar{\lambda}-1$ | $-\bar{\lambda}-2S-1$ | $1-2S$ | $-\bar{\lambda}-S-m$ | $-\bar{\lambda}-S+m$ |
| 2 | $-1+S$ | $S-m$ | $m+S$ | $-\bar{\lambda}-1$ | $-\bar{\lambda}+2S-1$ | $1+2S$ | $-\bar{\lambda}+S-m$ | $-\bar{\lambda}+S+m$ |
| 3 | $\bar{\lambda}-\lvert m\rvert$ | $-S-\lvert m\rvert$ | $S-\lvert m\rvert$ | $\bar{\lambda}+1$ | $\bar{\lambda}-2\lvert m\rvert+1$ | $1-2\lvert m\rvert$ | $\bar{\lambda}-S-\lvert m\rvert+2$ | $\bar{\lambda}+S-\lvert m\rvert+2$ |
| 4 | $\bar{\lambda}+\lvert m\rvert$ | $-S+\lvert m\rvert$ | $S+\lvert m\rvert$ | $\bar{\lambda}+1$ | $\bar{\lambda}+2\lvert m\rvert+1$ | $1+2\lvert m\rvert$ | $\bar{\lambda}-S+\lvert m\rvert+2$ | $\bar{\lambda}+S+\lvert m\rvert+2$ |

We have used the permutation invariance property to relabel the coefficients in an arbitrary manner.

The parameters for the four solutions around $1/R = 0$ ($R > 1$) are then

| $s$ | $\gamma_s$ | $a_1^s$ | $a_2^s$ | $a_3^s$ | $a_4^s$ | $b_1^s$ | $b_2^s$ | $b_3^s$ |
|---|---|---|---|---|---|---|---|---|
| 1 | $-\bar{\lambda} - S$ | $-S - m$ | $m - S$ | $-\bar{\lambda} - 1$ | $-\bar{\lambda} - 2S - 1$ | $1 - 2S$ | $-\bar{\lambda} - S - m$ | $-\bar{\lambda} - S + m$ |
| 2 | $-\bar{\lambda} + S$ | $S - m$ | $m + S$ | $-\bar{\lambda} - 1$ | $-\bar{\lambda} + 2S - 1$ | $1 + 2S$ | $-\bar{\lambda} + S - m$ | $-\bar{\lambda} + S + m$ |
| 3 | $1 - \|m\|$ | $-S - \|m\|$ | $S - \|m\|$ | $\bar{\lambda} + 1$ | $\bar{\lambda} - 2\|m\| + 1$ | $1 - 2\|m\|$ | $\bar{\lambda} - S - \|m\| + 2$ | $\bar{\lambda} + S - m + 2$ |
| 4 | $1 + \|m\|$ | $-S + \|m\|$ | $S + \|m\|$ | $\bar{\lambda} + 1$ | $\bar{\lambda} + 2\|m\| + 1$ | $1 + 2\|m\|$ | $\bar{\lambda} - S + \|m\| + 2$ | $\bar{\lambda} + S + \|m\| + 2$ |

Note that $\langle \hat{v}_m(r_1)\hat{v}_m^*(r_2)\rangle$ is symmetric with respect to the exchange of points 1 and 2 (exchanging $r_1 \leftrightarrow r_2$ and $\Delta\phi \to -\Delta\phi$). This implies the relation $f_m(R) = R^{\lambda} f_{-m}(1/R) = R^{\bar{\lambda}-1} f_{-m}(1/R)$. As expected, this symmetry is preserved: solutions $(1)-(4)$ for $R < 1$ are matched to solution $(1)-(4)$ with the variable $1/R' = R$ and $m' = -m$.

Note that solution (3) is not given by a Hypergeometric function as written in the table, since $m$ is integer so that solution (3) degenerates with solution (4) ($\gamma_3 - \gamma_4 = -2|m|$). Solution (3) is then a combination of solution (4) times $\ln R$ and a generalized power series starting with $R^{\bar{\lambda}-|m|}$. It is given by the Meijer G-function $G^{2,4}_{4,4}\left(R \,\middle|\, \begin{matrix} m, -m, \bar{\lambda} - S + 1, \bar{\lambda} + S + 1 \\ \bar{\lambda} - m, \bar{\lambda} + m, -S - 1, S - 1 \end{matrix}\right)$ [3].

The values that $\bar{\lambda}$ can take are limited by the requirement that the solution $\langle \hat{v}_m(r_1)\hat{v}_m^*(r_2)\rangle = r_1^{\lambda} f_m(r_2/r_1)$ satisfies the Cauchy-Schwarz inequality $|\langle \hat{v}_m(r_1)\hat{v}_m^*(r_2)\rangle| \le \sqrt{\langle |\hat{v}_m(r_1)|^2\rangle \langle |\hat{v}_m(r_2)|^2\rangle}$ for any $R$ and in particular for $R \to 0, \infty$. In principle we also need to check that $|\langle \hat{u}_{\pm m}(r_1)\hat{v}_{\mp m}(r_2)\rangle| \le \sqrt{\langle |\hat{u}_m(r_1)|^2\rangle \langle |\hat{v}_m(r_2)|^2\rangle}$. If we assume that the solution is dominated by a single solution out of $(1)-(4)$, we get the condition $R^{\gamma_i - (\bar{\lambda}-1)/2} / f_m^i(1) < 1$ for $R < 1$. Thus we have the condition $\bar{\lambda} \le 2\gamma_i + 1$ which gives: (1) $\bar{\lambda} \le -1 - 2S$; (2) $\bar{\lambda} \le -1 + 2S$; (3) $\bar{\lambda} \ge 2|m| - 1$; (4) $\bar{\lambda} \ge -2|m| - 1$ correspondingly for solutions $(1)-(4)$ in the table.

### 2. *Special cases*

For special values of the parameters the solution can reduce to polynomials, or become degenerate with another solution. The corresponding parameters for solutions 2 and 4 are:

- **Solution 2:** For $m > 1$ and $\bar{\lambda} = n - |m| + S$ with $n$ an integer and $n < |m| - 1 + S$, this solution is not defined as written in the table, since $\gamma_2$ differs by an integer multiple from $\gamma_4$ (and as a result $b_2$ leads to a divergence in one of the coefficients of the series).
  Instead, the solution is a combination of solution 4 multiplied by $\ln R$ and a Frobenius series with power $\gamma_2$. Another special case are the values $\bar{\lambda} = n - 1$ ($\lambda = n - 2$) with $n < 2S$ an integer, for which the Hypergeometric function reduces to a polynomial in $R$ of the order $\bar{\lambda} + 1$.

- **Solution 4:** For $m > 1$ there are polynomial solutions given by $\bar{\lambda} = -n - 1$ with $n > 0$ an integer such that $n \le 2|m|$.

## C. Explicit expressions and discussion of solutions for $|m| > 1$

Here we consider $|m| \neq 1$ since this is a degenerate case which we will explore separately (see section SII D). So, the solutions we get are:

- For $\bar{\lambda} \le -1 - 2\sqrt{m^2 - 1}$ and the parameters of line 1 in the table:

$$\langle \hat{v}_m(r_1)\hat{v}_m^*(r_2)\rangle = \begin{cases} A_m(\bar{\lambda}) r_1^{\bar{\lambda}-1} \left(\frac{r_2}{r_1}\right)^{-1-\sqrt{m^2-1}} {}_4F_3\left(a_1, a_2, a_3, a_4; b_1, b_2, b_3; \frac{r_2}{r_1}\right) & r_2 < r_1 \\ A_m(\bar{\lambda}) r_2^{\bar{\lambda}-1} \left(\frac{r_1}{r_2}\right)^{-1-\sqrt{m^2-1}} {}_4F_3\left(a_1, a_2, a_3, a_4; b_1, b_2, b_3; \frac{r_1}{r_2}\right) & r_2 > r_1 \end{cases}. \tag{S13}$$

- For $\bar\lambda \le -1+2\sqrt{m^2-1}$ and the parameters of line 2 in the table:

$$\langle \hat v_m(r_1)\hat v_m^*(r_2)\rangle = \begin{cases} A_m(\bar\lambda) r_1^{\bar\lambda-1}\left(\frac{r_2}{r_1}\right)^{-1+\sqrt{m^2-1}} {}_4F_3\left(a_1,a_2,a_3,a_4;b_1,b_2,b_3;\frac{r_2}{r_1}\right) & r_2<r_1 \\ A_m(\bar\lambda) r_2^{\bar\lambda-1}\left(\frac{r_1}{r_2}\right)^{-1+\sqrt{m^2-1}} {}_4F_3\left(a_1,a_2,a_3,a_4;b_1,b_2,b_3;\frac{r_1}{r_2}\right) & r_2>r_1 \end{cases}. \tag{S14}$$

- For $\bar\lambda \ge 2|m|-1$ :

$$\langle \hat v_m(r_1)\hat v_m^*(r_2)\rangle = \begin{cases} B_m(\bar\lambda) r_1^{\bar\lambda-1} G^{2,4}_{4,4}\left(R \left| \begin{matrix} m,-m,\bar\lambda-S+1,\bar\lambda+S+1 \\ \bar\lambda-m,\bar\lambda+m,-S-1,S-1\end{matrix}\right.\right) & r_2<r_1 \\ \\ B_m(\bar\lambda) r_2^{\bar\lambda-1} G^{2,4}_{4,4}\left(R \left| \begin{matrix} m,-m,\bar\lambda-S+1,\bar\lambda+S+1 \\ \bar\lambda-m,\bar\lambda+m,-S-1,S-1\end{matrix}\right.\right) & r_2>r_1 \end{cases}. \tag{S15}$$

- For $\bar\lambda \ge -2|m|-1$ and the parameters of line 4 in the table:

$$\langle \hat v_m(r_1)\hat v_m^*(r_2)\rangle = \begin{cases} B_m(\bar\lambda) r_1^{\bar\lambda-1}\left(\frac{r_2}{r_1}\right)^{\bar\lambda+|m|} {}_4F_3\left(a_1,a_2,a_3,a_4;b_1,b_2,b_3;\frac{r_2}{r_1}\right) & r_2<r_1 \\ B_m(\bar\lambda) r_2^{\bar\lambda-1}\left(\frac{r_1}{r_2}\right)^{\bar\lambda+|m|} {}_4F_3\left(a_1,a_2,a_3,a_4;b_1,b_2,b_3;\frac{r_1}{r_2}\right) & r_2>r_1 \end{cases}. \tag{S16}$$

Except for the polynomial solutions, these solutions generically have $\lim_{r_2\to r_1}\langle\hat\omega_m(r_1)\hat\omega_m^*(r_2)\rangle \to r^{\bar\lambda-1}/|r_1-r_2|$, a behavior which is cut off at $l_f$ so it is not a priori forbidden. Indeed, $\lim_{R\to 1} {}_4F_3\left(a_1,..,a_4;b_1..,b_3;R\right) \sim \Pi_{i=1}^3\Gamma(b_i)/\Pi_{i=1}^4\Gamma(a_i)(1-R)^3\ln(1-R)$ and the leading order term in this limit for the enstrophy comes from $\lim_{r_2\to r_1}\langle\hat\omega_m(r_1)\hat\omega_m^*(r_2)\rangle \to r^2\partial_{r_1}^2\partial_{r_2}^2\langle\hat v_m(r_1)\hat v_m^*(r_2)\rangle$.

**The limit $r_1\to r_2$:**

- For solution (2), with $\bar\lambda \le -1+2\sqrt{m^2-1}$ and the parameters of line 2 in the table we have

$$\langle \hat v_m(r)\hat v_m^*(r)\rangle = A_m(\bar\lambda) r^{\bar\lambda-1}\,{}_4F_3\left(a_1,..,a_4;b_1..,b_3;1\right), \tag{S17}$$

and

$$\langle \hat u_m(r_1)\hat v_m^*(r_2)\rangle = \begin{cases} \frac{i}{m}A_m r^{\bar\lambda-1}\left[(\bar\lambda+1-S)\,{}_4F_3\left(a_1,..,a_4;b_1..,b_3;1\right) - {}_4F_3'\left(a_1,..,a_4;b_1..,b_3;1\right)\right] & r_2\to r_1^- \\ \\ \frac{i}{m}A_m r^{\bar\lambda-1}\left[S\,{}_4F_3\left(a_1,..,a_4;b_1..,b_3;1\right) + {}_4F_3'\left(a_1,..,a_4;b_1..,b_3;1\right)\right] & r_2\to r_1^+ \end{cases}, \tag{S18}$$

where ${}_4F_3'\left(a_1,..,a_4;b_1..,b_3;1\right) = \partial_R\,{}_4F_3\left(a_1,a_2,a_3,a_4;b_1,b_2,b_3;R\right)_{R=1}$ and we see that in principle there might be a jump in $\langle u(r_1,\phi_1)v(r_2,\phi_2)\rangle$ depending on the side from which $r_2$ approaches $r_1$.

Finally the last velocity correlation function in this case is

$$\langle \hat u_m(r)\hat u_m^*(r)\rangle = -\frac{A_m(\bar\lambda)}{m^2} r^{\bar\lambda-1}\left[S(S-1-\bar\lambda)\,{}_4F_3\left(a_1,..,a_4;b_1..,b_3;1\right) + (2S-\bar\lambda)\,{}_4F_3'\left(a_1,..,a_4;b_1..,b_3;1\right) + {}_4F_3''\left(a_1,..,a_4;b_1..,b_3;1\right)\right]. \tag{S19}$$

- Solution (1) is obtained by replacing $S\to -S$ in the expressions for solution (2).
- Solution (4) with $\bar\lambda \ge -2|m|-1$ and the parameters of line 4 in the table is

$$\langle \hat u_m(r_1)\hat v_m^*(r_2)\rangle = \begin{cases} \frac{i}{m}B_m r^{\bar\lambda-1}\left[|m|\,{}_4F_3\left(a_1,..,a_4;b_1..,b_3;1\right) - {}_4F_3'\left(a_1,..,a_4;b_1..,b_3;1\right)\right] & r_2\to r_1^- \\ \\ \frac{i}{m}B_m r^{\bar\lambda-1}\left[(\bar\lambda+|m|+1)\,{}_4F_3\left(a_1,..,a_4;b_1..,b_3;1\right) + {}_4F_3'\left(a_1,..,a_4;b_1..,b_3;1\right)\right] & r_2\to r_1^+ \end{cases}. \tag{S20}$$

$$\langle \hat u_m(r)\hat u_m^*(r)\rangle = -\frac{B_m}{m^2}(\bar\lambda) r^{\bar\lambda-1}\left[|m|(|m|+1+\bar\lambda)\,{}_4F_3\left(a_1,..,a_4;b_1,..,b_3;1\right) + (2|m|+2+\bar\lambda)\,{}_4F_3'\left(a_1,..,a_4;b_1,..,b_3;1\right) + {}_4F_3''\left(a_1,..,a_4;b_1,..,b_3;1\right)\right] \tag{S21}$$

- We will not discuss solution (3) in detail here.

Let us discuss the jump in $\langle u(r_1,\phi_1)v(r_2,\phi_2)\rangle$, occurring depending on the side from which $r_2$ approaches $r_1$. It seems that this jump is absent for the polynomial (non constant) solutions (if $\exists i$ s.t $a_i = -n$, $n \in \mathbb{N}^+$). Such a jump implies that for $|r_1 - r_2| \sim O(l_f)$, $\langle u(r_1,\phi_1)v(r_2,\phi_2)\rangle$ is determined by the forcing in the main order. However, a balance between advection and forcing gives the estimate $\langle \hat{v}_m(r_1)\hat{v}^*_m(r_2)\rangle \propto \varepsilon r/(m^2 U)$ for $|r_1 - r_2| \leq l_f$ and $\langle |\hat{v}(r)|^2\rangle \propto \varepsilon r/U$. In fact, this is the theoretical result obtained for $\langle u(r)v(r)\rangle$, which we expect to be much smaller than $\langle |\hat{v}(r)|^2\rangle$ as is indeed observed in the simulations. Thus, solutions with a jump in $\langle u(r_1,\phi_1)v(r_2,\phi_2)\rangle$ cannot occur at leading order.

## D. Explicit expressions and discussion of solutions for $|m| = 1$

### 1. Solutions for generic $\bar{\lambda}$

Let us now discuss the solutions for $|m| = 1$; around $R = 0$ the four solutions are given by

$$\langle \hat{v}_{\pm 1}(r_1)\hat{v}_{\mp 1}(r_2)\rangle = \begin{cases} r_1^{\bar{\lambda}-1}\left((1-\bar{\lambda})\frac{r_1}{r_2} + 1 + \bar{\lambda}\right) \\ r_2^{\bar{\lambda}-1}((1-\bar{\lambda})\frac{r_2}{r_1} + 1 + \bar{\lambda}) \\ r_1^{\bar{\lambda}-1}\left((\frac{\lambda+1}{\lambda-1} - \frac{1}{R})\ln R + \frac{4-2\lambda^2}{(\lambda-1)^2} + \frac{\bar{\lambda}(\bar{\lambda}+1)}{2(1-\bar{\lambda})(2-\bar{\lambda})} R\, {}_3F_2(1,1,-\lambda+1,;3,-\lambda+3;\frac{r_2}{r_1}\right) \\ r_1^{\bar{\lambda}-1}\left(\frac{r_2}{r_1}\right)^{\bar{\lambda}+1} {}_3F_2(1,1,\lambda+1,;3,\lambda+3;\frac{r_2}{r_1}) \end{cases} \tag{S22}$$

where we have used $\sum_{n=2}^{\infty} \frac{(-\lambda-1)_n}{n(n-1)(1-\lambda)_n} R^{n-1} = R\frac{\bar{\lambda}(\bar{\lambda}+1)}{2(1-\bar{\lambda})(2-\bar{\lambda})}\, {}_3F_2(1,1,-\lambda+1,;3,-\lambda+3;R)$ for the third solution. The solutions around $1/R = 0$ are given by the above solutions with the replacement $r_1 \leftrightarrow r_2$. Here we have $\gamma = (-1, \lambda-1, -1, \lambda+1)$ and $\alpha = (0, 2, -\lambda, -\lambda)$. The third solution arises due to the degeneracy $\gamma_3 = \gamma_1 = -1$. On the other hand, the degeneracy $\gamma_4 - \gamma_2 = 2$ does not lead to a logarithmic solution. These solutions cover all cases except if $\lambda$ is an integer, in which case additional degeneracies of solutions can occur (between all four solutions). The values $\lambda = 1, -1$ are such special cases where some solutions become degenerate.

One can check explicitly that for the third and fourth solution the limit $r_1 \to r_2$ of $\langle \hat{v}_{\pm 1}(r_1)\hat{v}_{\mp 1}(r_2)\rangle$ depends on the direction, i.e there is a jump at $r_1 = r_2$. Therefore, these solutions cannot contribute to the leading order in the limit we are considering.

Let us write the first two allowed solutions in full for $\bar{\lambda} \neq 1, -1$:

$$\langle \hat{v}_{\pm 1}(r_1)\hat{v}_{\mp 1}(r_2)\rangle = \begin{cases} A_1(\bar{\lambda}) r_2^{\bar{\lambda}-1}((1-\bar{\lambda})\frac{r_2}{r_1} + 1 + \bar{\lambda}), & r_2 < r_1 \\ A_1(\bar{\lambda}) r_1^{\bar{\lambda}-1}\left((1-\bar{\lambda})\frac{r_1}{r_2} + 1 + \bar{\lambda}\right), & r_1 < r_2 \end{cases} \tag{S23}$$

$$\langle \hat{u}_{\pm 1}(r_1)\hat{v}_{\mp 1}(r_2)\rangle = \begin{cases} \frac{i}{m} A_1(\bar{\lambda}) r_2^{\bar{\lambda}-1}(1+\bar{\lambda}), & r_2 < r_1 \\ \frac{i}{m} A_1(\bar{\lambda}) r_1^{\bar{\lambda}-1}\left((1-\bar{\lambda}^2)\frac{r_1}{r_2} + \bar{\lambda} + \bar{\lambda}^2\right), & r_1 < r_2 \end{cases} \tag{S24}$$

$$\langle \hat{u}_{\pm 1}(r_1)\hat{u}_{\mp 1}(r_2)\rangle = \begin{cases} A_1(\bar{\lambda}) r_2^{\bar{\lambda}-1}\bar{\lambda}(1+\bar{\lambda}), & r_2 < r_1 \\ A_1(\bar{\lambda}) r_1^{\bar{\lambda}-1}\bar{\lambda}(1+\bar{\lambda}), & r_1 < r_2 \end{cases} \tag{S25}$$

and the Cauchy-Schwartz inequality gives the restriction $\bar{\lambda} > 1$. At $r_1 = r_2$ this gives:

$$\langle |\hat{v}_1(r)|^2\rangle = A_1(\bar{\lambda}) 2 r^{\bar{\lambda}-1}, \tag{S26}$$

$$\langle \hat{u}_{\pm 1}(r)\hat{v}_{\mp 1}(r)\rangle = \pm i A_1(\bar{\lambda}) r^{\bar{\lambda}-1}(1+\bar{\lambda}), \tag{S27}$$

$$\langle |\hat{u}_1(r)|^2\rangle = A_1(\bar{\lambda}) r^{\bar{\lambda}-1}\bar{\lambda}(1+\bar{\lambda}). \tag{S28}$$

The second family of solutions, corresponding to the first line in (S22) is given by the same expressions as above, interchanging $r_1 \to r_2$. With the restriction $\bar{\lambda} < -1$ from the Cauchy-Schwartz inequality.

### 2. Solutions for $\bar{\lambda} = 1$

Let us write separately the solutions for $\bar{\lambda} = 1$. We only consider the first three solution; $\bar{\lambda} = 1$ is not special for the fourth. In addition to a constant solution, $\langle \hat{v}_{\pm 1}(r_1)\hat{v}_{\mp 1}(r_2)\rangle = \langle \hat{u}_{\pm 1}(r_1)\hat{u}_{\mp 1}(r_2)\rangle = |\langle \hat{v}_{\pm 1}(r_1)\hat{u}_{\mp 1}(r_2)\rangle| = \text{Const}$,

there is the solution:

$$\langle \hat{v}_{\pm 1}(r_1)\hat{v}_{\mp 1}(r_2)\rangle = \begin{cases} C_1(1)(-1/R + R - 2\log R), & r_2 < r_1 \\ C_1(1)(1/R - R + 2\log R), & r_1 < r_2 \end{cases} \tag{S29}$$

which vanishes at $R = 1$. Also $\langle \hat{v}_{\pm 1}(r)\hat{u}_{\mp 1}(r)\rangle = \langle \hat{u}_{\pm 1}(r)\hat{u}_{\mp 1}(r)\rangle = 0$ for this solution. Therefore, we cannot detect its presence from single point harmonics. The other solution is given by

$$\langle \hat{v}_{\pm 1}(r_1)\hat{v}_{\mp 1}(r_2)\rangle = \begin{cases} D_1(1)[5R + (-5 + 1/R - R)\log R + (\log R)^2], & r_2 < r_1 \\ D_1(1)[5/R - (-5 - 1/R + R)\log R + (\log R)^2], & r_1 < r_2 \end{cases} \tag{S30}$$

which gives

$$\langle |\hat{v}_1(r)|^2\rangle = 5D_1(1), \tag{S31}$$

$$\langle \hat{u}_{\pm 1}(r)\hat{v}_{\mp 1}(r)\rangle = \pm i5D_1(1), \tag{S32}$$

$$\langle |\hat{u}_1(r)|^2\rangle = 2D_1(1). \tag{S33}$$

### *3. Solutions for $\bar{\lambda} = -1$*

The solutions for $\bar{\lambda} = -1$ are:

- First,

$$\langle \hat{v}_{\pm 1}(r_1)\hat{v}_{\mp 1}(r_2)\rangle = \begin{cases} C_1(-1)r_1^{-2}, & r_2 < r_1 \\ C_1(-1)r_2^{-2}, & r_1 < r_2 \end{cases}, \tag{S34}$$

  which gives

$$\langle |\hat{v}_1(r)|^2\rangle = C_1(-1)r^{-2}, \tag{S35}$$

$$\langle \hat{u}_{\pm 1}(r_1)\hat{v}_{\mp 1}(r_2)\rangle = \begin{cases} \mp iC_1(-1)r_1^{-2} & r_2 < r_1 \\ \pm iC_1(-1)r_2^{-2}, & r_1 < r_2 \end{cases}, \tag{S36}$$

$$\langle |\hat{u}_1(r)|^2\rangle = -C_1(-1)r^{-2}. \tag{S37}$$

- Second,

$$\langle \hat{v}_{\pm 1}(r_1)\hat{v}_{\mp 1}(r_2)\rangle = \begin{cases} D_1(-1)r_2^{-2}, & r_2 < r_1 \\ D_1(-1)r_1^{-2}, & r_1 < r_2 \end{cases}, \tag{S38}$$

  which gives

$$\langle |\hat{v}_1(r)|^2\rangle = D_1(-1)r^{-2}, \tag{S39}$$

$$\langle \hat{u}_{\pm 1}(r_1)\hat{v}_{\mp 1}(r_2)\rangle = \begin{cases} \pm iD_1(-1)r_2^{-2} & r_2 < r_1 \\ \mp iD_1(-1)r_1^{-2}, & r_1 < r_2 \end{cases}, \tag{S40}$$

$$\langle |\hat{u}_1(r)|^2\rangle = -D_1(-1)r^{-2}, \tag{S41}$$

  but does not satisfy the Cauchy-Schwartz inequality.

- Third,

$$\langle \hat{v}_{\pm 1}(r_1)\hat{v}_{\mp 1}(r_2)\rangle = \frac{A_1(-1)}{r_1 r_2}, \tag{S42}$$

  which gives

$$\langle |\hat{v}_1(r)|^2\rangle = A_1(-1)r^{-2}, \tag{S43}$$

$$\langle \hat{u}_{\pm 1}(r_1)\hat{v}_{\mp 1}(r_2)\rangle = 0, \tag{S44}$$

$$\langle \hat{u}_{\pm 1}(r_1)\hat{u}_{\mp 1}(r_2)\rangle = 0. \tag{S45}$$

- Fourth,

$$\langle \hat{v}_{\pm 1}(r_1)\hat{v}_{\mp 1}(r_2)\rangle = \begin{cases} \frac{E_1(-1)}{r_1 r_2}(1+\ln(r_2/r_1)), & r_2 < r_1 \\ \frac{E_1(-1)}{r_1 r_2}(1-\ln(r_2/r_1)), & r_1 < r_2 \end{cases}, \tag{S46}$$

which gives

$$\langle |\hat{v}_1(r)|^2\rangle = E_1(-1) r^{-2}, \tag{S47}$$

$$\langle \hat{u}_{\pm 1}(r_1)\hat{v}_{\mp 1}(r_2)\rangle = \begin{cases} \mp i E_1(-1) r_2^{-2} & r_2 < r_1 \\ \pm i E_1(-1) r_1^{-2}, & r_1 < r_2 \end{cases}, \tag{S48}$$

$$\langle \hat{u}_{\pm 1}(r_1)\hat{u}_{\mp 1}(r_2)\rangle = 0. \tag{S49}$$

### E. Identification of solutions combining numerics and theory for $m = 1$ modes

The numerical results in Fig. S3 indicate that in the universal region $\langle |\hat{u}_1|^2\rangle \approx$ Const, $\langle \hat{u}_1\hat{v}_{-1}\rangle \approx$ Const while $\langle |\hat{v}_1|^2\rangle \approx r^{-\beta}$ with some $\beta > 0$. Therefore, we search for solution that are a superposition of a constant and a power law which does not contribute to $\langle |\hat{u}_1|^2\rangle \approx$ Const, $\langle \hat{u}_1\hat{v}_{-1}\rangle \approx$ Const. There are two solution which correspond to $\bar{\lambda} = 1$ for $m = 1$, so that the constant part of the solution is given by:

$$\langle |\hat{v}_1(r)|^2\rangle = A_1(1) + 5D_1(1), \tag{S50}$$

$$\langle |\hat{u}_1(r)|^2\rangle = A_1(1) + 2D_1(1), \tag{S51}$$

$$\langle \hat{u}_{\pm 1}(r)\hat{v}_{\mp 1}(r)\rangle = \pm i(A_1(1) + 5D_1(1)). \tag{S52}$$

The requirement $|\langle \hat{u}_{\pm 1}(r)\hat{v}_{\mp 1}(r)\rangle| \le \sqrt{\langle |\hat{u}_{\pm 1}(r)|^2\rangle\langle |\hat{v}_{\pm 1}(r)|^2\rangle}$ necessitates that $D_1 \le 0$. The numerical simulations, however, imply that $\langle |\hat{u}_1|^2\rangle = |\langle \hat{u}_1\hat{v}_{-1}\rangle|$ so that $D_1 = 0$.

Next, let us consider which $\bar{\lambda}$ give a solution with $\langle |\hat{u}_1|^2\rangle = 0$ and $\langle \hat{u}_1\hat{v}_{-1}\rangle = 0$: this is only solution $A_1(\bar{\lambda})$ with $\bar{\lambda} = -1$ if we discard the third and fourth solutions for $\bar{\lambda} \neq \pm 1$, since they contain a jump for $\langle \hat{u}_1\hat{v}_1^*\rangle$ (note that a superposition of solutions one and two , with the same $\bar{\lambda} = \pm 1$ cannot give $\langle |\hat{u}_1|^2\rangle = \langle \hat{u}_1\hat{v}_{-1}\rangle = 0$ without $\langle |\hat{v}_1|^2\rangle = 0$).

Then we have

$$\langle |\hat{v}_1(r)|^2\rangle = A_1(1) + A_1(-1)\left(\frac{l_f}{r}\right)^2, \tag{S53}$$

$$\langle |\hat{u}_1(r)|^2\rangle = A_1(1), \tag{S54}$$

$$\langle \hat{u}_{\pm 1}(r)\hat{v}_{\mp 1}(r)\rangle = \pm i A_1(1). \tag{S55}$$

Note that the Cauchy-Schwartz inequality is satisfied for these solutions: we require that

$$\left| A_1(1) - A_1(-1)\left(\frac{l_f}{r_2}\right)^2 \frac{r_2}{r_1}\right| \le \sqrt{\left(A_1(1) + A_1(-1)\left(\frac{l_f}{r_1}\right)^2\right)\left(A_1(1) + A_1(-1)\left(\frac{l_f}{r_2}\right)^2\right)} \tag{S56}$$

for $l_f < r_2 < r_1 < L$.

### F. Identification of solutions combining numerics and theory for $m = 2$ modes

The numerical results in Fig. S3 indicate that $\langle \hat{u}_2\hat{v}_{-2}\rangle \approx Const$ implying that $\bar{\lambda} = 1$ gives a contribution to this mode as well. The only solution for which $\bar{\lambda} = 1$ is in the range of validity and has a non-zero $\langle \hat{u}_2\hat{v}_{-2}\rangle$ (and without a jump) is solution (2) in the table. For $\bar{\lambda} = 1$ this solution is a polynomial of degree two. This solution has

$$\frac{\langle |\hat{u}_2(r)|^2\rangle}{\langle |\hat{v}_2(r)|^2\rangle} = \frac{19}{28}, \tag{S57}$$

and

$$\frac{\Im\langle \hat{u}_{\pm 2}(r)\hat{v}_{\mp 2}(r)\rangle}{\langle |\hat{v}_2(r)|^2\rangle} = \frac{1}{2}. \tag{S58}$$

Let us check if $\bar{\lambda} = -1$ could contribute to $m = 2$ as well as $m = 1$. From DNS we expect that $\langle|\hat{v}_2(r)|^2\rangle = A_2(1) - A_2(-1)r^{-2}$. The two options which satisfy the Cauchy-Schwartz inequality for such a $\bar{\lambda}$ are (2), (4). Solution (2) gives

$$\langle \hat{v}_{\pm 2}(r_1)\hat{v}_{\mp 2}(r_2)\rangle = \begin{cases} A_2(-1) r_1^{-1-\sqrt{3}} r_2^{-1+\sqrt{3}}, & r_2 < r_1 \\ A_2(-1) r_2^{-1-\sqrt{3}} r_1^{-1+\sqrt{3}}, & r_1 < r_2 \end{cases}, \tag{S59}$$

$$\langle|\hat{v}_2(r)|^2\rangle = A_2(-1) r^{-2}, \tag{S60}$$

and

$$\langle \hat{u}_{\pm 2}(r_1)\hat{v}_{\mp 2}(r_2)\rangle = \begin{cases} \mp i A_2(-1)\frac{\sqrt{3}}{2} r_1^{-1-\sqrt{3}} r_2^{-1+\sqrt{3}}, & r_2 < r_1 \\ \pm i A_2(-1)\frac{\sqrt{3}}{2} r_2^{-1-\sqrt{3}} r_1^{-1+\sqrt{3}}, & r_1 < r_2 \end{cases}, \tag{S61}$$

$$\langle|\hat{u}_2(r)|^2\rangle = -\frac{3}{4} A_2(-1) r^{-2}. \tag{S62}$$

Solution (4) gives

$$\langle \hat{v}_{\pm 2}(r_1)\hat{v}_{\mp 2}(r_2)\rangle = \begin{cases} B_2(-1) r_1^{-3} r_2, & r_2 < r_1 \\ B_2(-1) r_2^{-3} r_1, & r_1 < r_2 \end{cases}, \tag{S63}$$

$$\langle|\hat{v}_2(r)|^2\rangle = B_2(-1) r^{-2}, \tag{S64}$$

and

$$\langle \hat{u}_{\pm 2}(r_1)\hat{v}_{\mp 2}(r_2)\rangle = \begin{cases} \mp i B_2(-1) r_1^{-3} r_2, & r_2 < r_1 \\ \pm i B_2(-1) r_2^{-3} r_1, & r_1 < r_2 \end{cases}, \tag{S65}$$

$$\langle|\hat{u}_2(r)|^2\rangle = -B_2(-1) r^{-2}. \tag{S66}$$

Now, to avoid a jump of $\langle \hat{v}_{\pm 2}(r_1)\hat{v}_{\mp 2}(r_2)\rangle$ and to make it zero we can take the combination

$$\langle \hat{v}_{\pm 2}(r_1)\hat{v}_{\mp 2}(r_2)\rangle = \begin{cases} \frac{A_2(-1)}{r_1 r_2}\left[\left(\frac{r_2}{r_1}\right)^{\sqrt{3}} - \frac{\sqrt{3}}{2}\left(\frac{r_2}{r_1}\right)^2\right], & r_2 < r_1 \\ \frac{A_2(-1)}{r_1 r_2}\left[\left(\frac{r_1}{r_2}\right)^{\sqrt{3}} - \frac{\sqrt{3}}{2}\left(\frac{r_1}{r_2}\right)^2\right], & r_1 < r_2 \end{cases}, \tag{S67}$$

$$\langle|\hat{v}_2(r)|^2\rangle = A_2(-1)\left(1 - \frac{\sqrt{3}}{2}\right) r^{-2}, \tag{S68}$$

and

$$\langle \hat{u}_{\pm 2}(r_1)\hat{v}_{\mp 2}(r_2)\rangle = \begin{cases} \mp i \frac{A_2(-1)}{r_1 r_2}\frac{\sqrt{3}}{2}\left[\left(\frac{r_2}{r_1}\right)^{\sqrt{3}} - \left(\frac{r_2}{r_1}\right)^2\right], & r_2 < r_1 \\ \pm i \frac{A_2(-1)}{r_1 r_2}\frac{\sqrt{3}}{2}\left[\left(\frac{r_1}{r_2}\right)^{\sqrt{3}} - \left(\frac{r_1}{r_2}\right)^2\right], & r_1 < r_2 \end{cases}, \tag{S69}$$

$$\langle|\hat{u}_2(r)|^2\rangle = (\frac{\sqrt{3}}{2} - \frac{3}{4}) A_2(-1) r^{-2}, \tag{S70}$$

which is consistent with taking $A_2(-1) > 0$ and having a positive contribution to $\langle|\hat{u}_2(r)|^2\rangle$ and $\langle|\hat{v}_2(r)|^2\rangle$.

The combination of the constant and $r^{-2}$ solutions yields Eq. (7) in the main text; in addition to the tests of this theoretical solution against the DNS data presented there (see Fig. 5 in the main text), we show in Fig. S4 the combination $\langle|\hat{v}_2|^2\rangle - 2\Im\langle\hat{u}_2\hat{v}_2^*\rangle$, rescaled properly, which exhibits the $r^{-2}$ contribution to $\langle|\hat{v}_2|^2\rangle$.

## SIII. ZEROTH ANGULAR HARMONIC

The zeroth harmonic ($m = 0$ mode) is not determined by the advection operator which gives the leading order contribution for the higher harmonics. It is is non-zero only for $\langle u_1 u_2\rangle$ (we require that $\nabla \cdot \mathbf{f} = 0$ implying that $\int \chi_{12}^{rr} d\phi = 0$ just like $\int v d\phi = 0$).

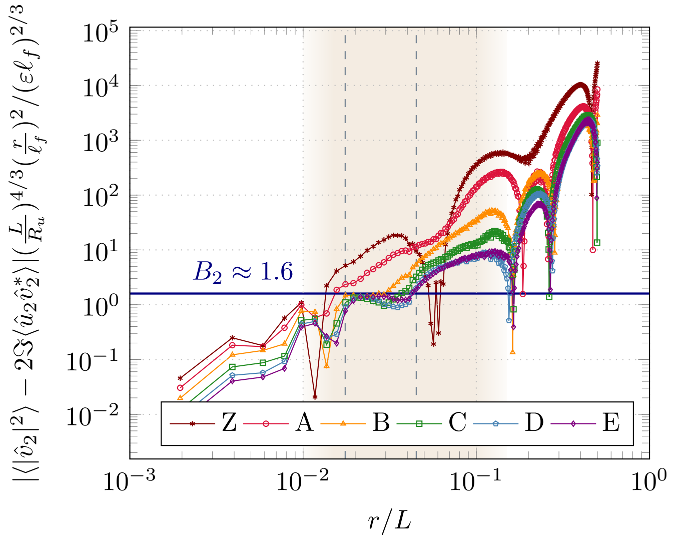


FIG. S4. Combination of the second harmonics evidencing the $r^{-2}$ contribution to the profile of $\langle|\hat{v}_2|^2\rangle$.

Let us write the equation for the fluctuations in the $\phi$ direction. We use the relation

$$(\tilde{\mathbf{v}}^l\nabla^l\tilde{\mathbf{v}})_\phi = v\partial_r u + \frac{u}{r}\partial_\phi u + \frac{uv}{r} = \frac{1}{r^2}\partial_r(r^2 uv) + \frac{1}{r}\partial_\phi u^2, \tag{S71}$$

so that the resulting equation for $\Gamma \ll 1$ is:

$$\frac{1}{r_1}\partial_{r_2} r_2\langle p_1 v_2\rangle + \frac{1}{r_2}\partial_{r_1} r_1\langle p_2 v_1\rangle - 2\chi_{12}^{\phi\phi} + 2\alpha\langle u_1 u_2\rangle = -\frac{1}{r_1^2}\partial_{r_1} r_1^2\langle v_1 u_1 u_2\rangle - \frac{1}{r_1}\partial_{\phi_1}\langle u_1^2 u_2\rangle - \frac{1}{r_2^2}\partial_{r_2} r_2^2\langle v_2 u_1 u_2\rangle \\ -\frac{1}{r_2}\partial_{\phi_2}\langle u_1 u_2^2\rangle + U\partial_{r_1}\langle u_2 v_1\rangle + U\partial_{r_2}\langle u_1 v_2\rangle. \tag{S72}$$

Then, integrating with respect to $\phi$ at $r_1 = r_2$, we have

$$\langle|\hat{u}_0|^2\rangle = \frac{1}{\alpha}\int_0^{2\pi}\chi_{12}^{\phi\phi} d\Delta\phi - \frac{1}{2\alpha}\int_0^{2\pi}\frac{1}{r^2}\partial_r r^2\langle(v_1+v_2)u_1u_2\rangle d\Delta\phi. \tag{S73}$$

Let us assume that $r \gg l_f$. For the forcing term we may safely use the approximation that it is equal to $\varepsilon$ for $\delta r \le l_f$ and is zero for $\delta r > l_f$. The upper limit of the integration is then determined by $\delta r \approx r\Delta\phi = l_f$ and after integration one gets the estimate $\varepsilon l_f/r$.

It isn't entirely clear what would be a correct estimate for the non-linear term, and how it would compare to the dissipation. Note that above we have assumed that $\Gamma \ll 1$ for the dissipation, which is not the case in the simulations. In any case, there is a question if the injection by forcing is balanced by the non-linear interactions or by dissipation, as assumed in [4]. In the simulations, Fig. S5, the zeroth harmonic varies with the different runs, which may be the result of $\Gamma$ increasing as $\alpha$ is decreasing while viscosity is kept fixed. Thus, it seems that the zeroth harmonic is sensitive to the dissipation mechanism at the forcing scale, unlike the higher harmonics and the energy.


[1] J. Laurie, G. Boffetta, G. Falkovich, I. Kolokolov, and V. Lebedev, Phys. Rev. Lett. **113**, 254503 (2014).
[2] N. E. Norlund, Acta Math. **94**, 289 (1955).
[3] A. M. Mathai and R. K. Saxena, *Generalized hypergeometric functions with applications in statistics and physical sciences* (Springer, 1973).
[4] I. V. Kolokolov and V. V. Lebedev, J. Fluid Mech. **809**, R2 (2016).

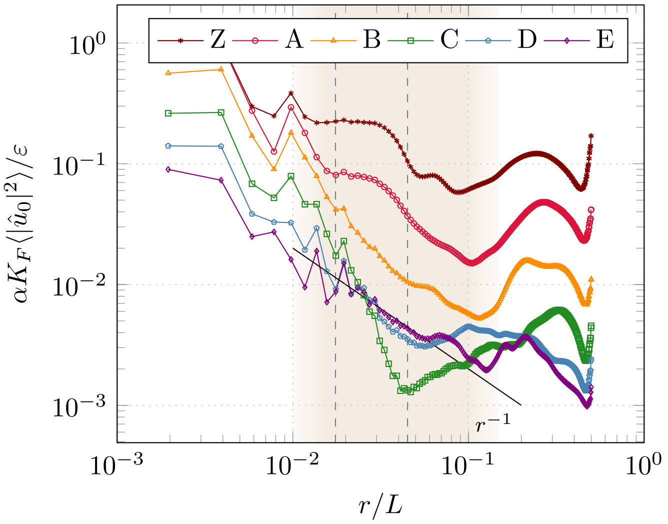


FIG. S5. (color online) Profile of the zeroth harmonics ($m = 0$) of turbulent energy, for all the runs.
